# Supplementary material for: On Explicit Super-Expressive Approximation for Neural Networks
Source: arXiv:2607.06781 source file (2026-07-07)
Supplement: Supplementary file 1 [file 08_Appendix.tex]

\appendix

\section{Prime estimates for CRT parameters and addressing costs}
\label{app:prime-estimates}

This appendix records the elementary prime estimates used in
Section~\ref{sec:symbolic}.  Their only role is to support the
decoder-aware memory bounds for CRT parameters and table-addressed
modulus assignments.  No number-theoretic optimality is needed.

Throughout this appendix, let \(p_n\) denote the \(n\)-th prime number,
and let
\[
\pi(q):=\#\{p\ \text{prime}:p\le q\}
\]
be the prime-counting function.  We use the convention \(\pi(1)=0\).  We use only the coarse consequence \(p_n=O(n\log n)\), or more explicitly
\(p_n\le Cn(\log n+\log\log n)\).  Such estimates go back to
\cite{rosser1962approximate} and are sharpened in later work of \cite{dusart2010estimates}.

\begin{lemma}[A standard upper bound for prime growth]
\label{lem:prime-growth-upper}
BThere exists a universal constant \(C_{\rm pr}>0\) such that, for every
\(n\ge 1\),
\[
p_n \le C_{\rm pr}\, n\log(n+1).
\]
Consequently, for every \(q\ge 1\) and \(K\ge 1\),
\[
\log_2 p_{\pi(q)+K}
\le
C_{\rm pr}'\bigl(\log_2(q+2)+\log_2(K+1)\bigr)
\]
for a universal constant \(C_{\rm pr}'>0\).
\end{lemma}

\begin{proof}
The first estimate is a standard consequence of classical bounds on the
\(n\)-th prime.  For example, one may use the elementary form
\(p_n\le C n\log(n+1)\) for a universal constant \(C\).

For the second estimate, observe that \(\pi(q)\le q\).  Hence
\[
\pi(q)+K \le q+K.
\]
Applying the first estimate gives
\[
p_{\pi(q)+K}
\le
C_{\rm pr}(q+K)\log(q+K+1).
\]
Taking base-two logarithms and using
\[
\log(q+K+1)
\le
\log(q+2)+\log(K+1)
\]
up to a universal additive constant yields the stated bound.
\end{proof}

\begin{lemma}[Canonical prime assignment]
\label{lem:canonical-prime-assignment}
Fix \(q\in\mathbb N_+\) and an ordering
\[
\Lambda_m=\{\nu(1),\dots,\nu(K)\}.
\]
Define
\[
p_{\nu(j)}:=p_{\pi(q)+j},
\qquad j=1,\dots,K.
\]
Then the integers \(\{p_\nu\}_{\nu\in\Lambda_m}\) are pairwise coprime,
satisfy
\[
p_\nu>q
\qquad
\forall \nu\in\Lambda_m,
\]
and obey the uniform logarithmic estimate
\[
\sum_{\nu\in\Lambda_m}\log_2 p_\nu
\le
C_{\rm can}\,
K\bigl(\log_2(q+2)+\log_2(K+1)\bigr)
\]
for a universal constant \(C_{\rm can}>0\).
\end{lemma}

\begin{proof}
The integers \(p_{\nu(j)}\) are distinct primes, hence pairwise coprime.
Since \(p_{\pi(q)+1}\) is the first prime strictly larger than \(q\), each
\(p_{\nu(j)}\) is larger than \(q\).

For the logarithmic estimate, monotonicity of \(p_n\) gives
\[
p_{\nu(j)}
=
p_{\pi(q)+j}
\le
p_{\pi(q)+K}
\qquad
\forall j=1,\dots,K.
\]
Therefore
\[
\sum_{\nu\in\Lambda_m}\log_2 p_\nu
\le
K\log_2 p_{\pi(q)+K}.
\]
The conclusion follows from Lemma~\ref{lem:prime-growth-upper}.
\end{proof}

\begin{lemma}[Lower bound for table-addressed coprime moduli]
\label{lem:table-address-lower}
Let \(\{m_\nu\}_{\nu\in\Lambda_m}\) be pairwise coprime integers greater
than \(1\).  Then there exists a universal constant \(c_{\rm tab}>0\)
such that, for all \(K\ge 2\),
\[
\sum_{\nu\in\Lambda_m}\log_2 m_\nu
\ge
c_{\rm tab}K\log_2 K.
\]
Consequently,
\[
\sum_{\nu\in\Lambda_m}\lceil \log_2 m_\nu\rceil
\ge
c_{\rm tab}K\log_2 K.
\]
\end{lemma}

\begin{proof}
For each \(\nu\), choose a prime divisor \(r_\nu\) of \(m_\nu\).  Since the
integers \(m_\nu\) are pairwise coprime, the chosen primes \(r_\nu\) are
distinct.  After sorting these primes increasingly, the \(j\)-th selected
prime is at least \(p_j\).  Hence
\[
\sum_{\nu\in\Lambda_m}\log_2 m_\nu
\ge
\sum_{\nu\in\Lambda_m}\log_2 r_\nu
\ge
\sum_{j=1}^K \log_2 p_j.
\]
Since \(p_j\ge j+1\), we have
\[
\sum_{j=1}^K \log_2 p_j
\ge
\sum_{j=1}^K \log_2(j+1)
=
\log_2((K+1)!).
\]
By Stirling's lower bound, or by the elementary inequality
\((K+1)!\ge (K/2)^{K/2}\) for \(K\ge 2\), this is bounded below by
\(c_{\rm tab}K\log_2 K\) after adjusting the universal constant.
The ceiling version follows because
\(\lceil\log_2 m_\nu\rceil\ge \log_2 m_\nu\).
\end{proof}

\begin{proof}[Proof of Corollary~\ref{cor:holder-smooth}]
Fix $\varepsilon\in(0,\tfrac12]$; the range $\varepsilon\in(\tfrac12,1)$ is covered below. Write
$L:=\log_2(1/\varepsilon)$ and $N:=\binom{D+r}{r}$, and assume $r\ge1$ (for $r=0$ the bound
$|f(x)-f(x_{\mathbf m})|\le AM^{-\gamma}$ gives the Hölder-$0$ analogue directly). Partition
$\Omega$ into $M^D$ grids with corners $x_{\mathbf m}=\mathbf m/M$ and local coordinate
$z:=M(x-x_{\mathbf m})\in[0,1)^D$; the value of $M$ is fixed in Step~1. We approximate $f$ on each
grid by a rationalised Taylor polynomial; the resulting $\tilde f$ is a rational gridwise polynomial,
realised exactly by Theorem~\ref{thm:main-theorem2}, whose architecture (activations, width
$\max\{2D,D+5N+1\}$, depth $r+15$) is independent of $M$, hence of $\varepsilon$ and $f$.

\smallskip
\noindent\textbf{Step 1 (Taylor error).} Let $T_{\mathbf m}$ be the degree-$r$ Taylor polynomial of $f$
at $x_{\mathbf m}$. Its integral remainder is
\[
f(x)-T_{\mathbf m}(x)=\sum_{|\alpha|=r}\frac{r}{\alpha!}(x-x_{\mathbf m})^{\alpha}\!\int_0^1(1-t)^{r-1}
\big[\partial^\alpha f(x_{\mathbf m}+t(x-x_{\mathbf m}))-\partial^\alpha f(x_{\mathbf m})\big]\,dt .
\]
On $\Omega_{\mathbf m}$, $\|x-x_{\mathbf m}\|_\infty\le 1/M$, so with $|\partial^\alpha f(x_{\mathbf m}+t\cdot)-
\partial^\alpha f(x_{\mathbf m})|\le A\,t^\gamma\|x-x_{\mathbf m}\|_\infty^\gamma$ and $|(x-x_{\mathbf m})^\alpha|
\le\|x-x_{\mathbf m}\|_\infty^{r}$,
\[
|f(x)-T_{\mathbf m}(x)|\le A\,M^{-(r+\gamma)}\,r\,B(\gamma+1,r)\sum_{|\alpha|=r}\tfrac1{\alpha!}
=A\,M^{-(r+\gamma)}\,\frac{D^{r}\Gamma(\gamma+1)}{\Gamma(r+\gamma+1)}=:C_{D,r,\gamma}A\,M^{-(r+\gamma)},
\]
using $r\,B(\gamma+1,r)=\Gamma(\gamma+1)r!/\Gamma(r+\gamma+1)$ and $\sum_{|\alpha|=r}1/\alpha!=D^r/r!$.
Requiring $C_{D,r,\gamma}A\,M^{-(r+\gamma)}\le\varepsilon/2$, set
\[
\kappa:=\Big(\tfrac{2D^{r}\Gamma(\gamma+1)}{\Gamma(r+\gamma+1)}A\Big)^{1/(r+\gamma)},\qquad
M:=\big\lceil\kappa\,\varepsilon^{-1/(r+\gamma)}\big\rceil\le(1+\kappa)\,\varepsilon^{-1/(r+\gamma)},
\]
so that the Taylor error is $\le\varepsilon/2$ and $M^{2D}\le(1+\kappa)^{2D}\varepsilon^{-2D/(r+\gamma)}$.

\smallskip
\noindent\textbf{Step 2 (rationalisation at fixed bit length).} In the local coordinate $z$ the
polynomial reads $\sum_{i\le N}c_{\mathbf m,i}z^{\alpha^{(i)}}$; the exact coefficients of $T_{\mathbf m}$ are
\[
c^\star_{\mathbf m,i}=\frac{\partial^{\alpha^{(i)}}f(x_{\mathbf m})}{\alpha^{(i)}!\,M^{|\alpha^{(i)}|}},
\qquad |c^\star_{\mathbf m,i}|\le B .
\]
Round each to the common dyadic precision $2^{-q}$ with $q:=\lceil\log_2(N/\varepsilon)\rceil\ (\ge1)$:
\[
c_{\mathbf m,i}:=2^{-q}\big\lfloor 2^{q}c^\star_{\mathbf m,i}+\tfrac12\big\rfloor,\qquad
|c_{\mathbf m,i}-c^\star_{\mathbf m,i}|\le 2^{-q-1}\le\tfrac{\varepsilon}{2N}.
\]
Since $|z^{\alpha^{(i)}}|\le1$, the per-grid rationalisation error is $\le N\cdot\tfrac{\varepsilon}{2N}=\varepsilon/2$,
hence $\|\tilde f-f\|_\infty\le\varepsilon$. In lowest terms $c_{\mathbf m,i}=s_{\mathbf m,i}/g_{\mathbf m,i}$ with
$g_{\mathbf m,i}\mid 2^{q}$, so $g_{\mathbf m,i}\le 2^{q}$ and $|s_{\mathbf m,i}|\le(B+1)2^{q}$. By
Definition~\ref{def:rational-bit-length} (using $q\ge1$),
\[
F:=\max_{\mathbf m,i}\operatorname{bits}(c_{\mathbf m,i})
\le\big(q+\log_2(B+2)+1\big)+\big(q+1\big)=2q+\log_2(B+2)+2
\le 2L+2\log_2 N+\log_2(B+2)+4,
\]
a bound uniform over all $M^DN$ coefficients and depending only on $B,N,\varepsilon$.

\smallskip
\noindent\textbf{Step 3 (parameter bound).} As $\tilde f$ is a degree-$\le r$ rational gridwise polynomial
with coefficient bit length $\le F$, Theorem~\ref{thm:main-theorem2} (Eq.~(59), $r\ge1$) gives
$\log_2\mathcal P(\Psi_\varepsilon)\le 2M^{2D}(D\log_2 M+FN)$. With
$\log_2 M\le\log_2(1+\kappa)+\tfrac{L}{r+\gamma}$ and the bound on $F$,
\[
D\log_2 M+FN\le \tfrac{D}{r+\gamma}L+2NL+D\log_2(1+\kappa)+2N\log_2 N+N\log_2(B+2)+4N.
\]
For $\varepsilon\le\tfrac12$ we have $L\ge1$, so each $L$-free term is at most that term times $L$, whence
\[
D\log_2 M+FN\le L\Big[\tfrac{D}{r+\gamma}+D\log_2(1+\kappa)+2N\log_2 N+N\log_2(B+2)+6N\Big].
\]
Multiplying by $2M^{2D}\le 2(1+\kappa)^{2D}\varepsilon^{-2D/(r+\gamma)}$ and absorbing the first two terms
under $N$ ($N\ge1$),
\[
\log_2\mathcal P(\Psi_\varepsilon)\le \tilde C_{D,r,\gamma,A,B}\,\varepsilon^{-2D/(r+\gamma)}\log_2(1/\varepsilon),
\]
\[
\tilde C_{D,r,\gamma,A,B}=2(1+\kappa)^{2D}\binom{D+r}{r}\Big[6+2\log_2\!\tbinom{D+r}{r}+\log_2(B+2)
+D\log_2(1+\kappa)+\tfrac{D}{r+\gamma}\Big].
\]
For $\varepsilon\in(\tfrac12,1)$ the same computation holds with $\log_2(1/\varepsilon)$ replaced by
$\max\{1,\log_2(1/\varepsilon)\}$; equivalently one retains the additive constants displayed above.
\end{proof}
